# Supplementary material for: Action-conditioned On-demand Motion Generation
Source: arXiv:2207.08164 source file (2022-07-17)
Supplement: Supplementary file 1 [file mm_sampling.tex]

\begin{table}[!ht]
\footnotesize
\centering
\caption{\label{tab:mm_humanact}Benchmark for MM on three  Dataset based on classifier.}
\begin{tabular}{@{}lcccc@{}}
\toprule
&\multicolumn{4}{c}{HumanAct12}   \\ \midrule
Methods                     & Acc$\uparrow$        & FID$\downarrow$     & Diversity          & MModality                   \\ \midrule
Real motions                & $\mstd{99.70}{.06}$  & $\mstd{0.02}{.01}$  & $\mstd{7.08}{.06}$ & $\mstd{2.53}{.05}$  \\ \midrule
ODMO                        & $\mstd{98.57}{.32}$  & $\mstd{0.07}{.00}$  & $\mstd{6.99}{.07}$ & $\mstd{2.50}{.05}$  \\
ODMO$_{\text{MM}}$                        & $\mstd{97.63}{.30}$  & $\mstd{0.15}{.02}$  & $\mstd{7.11}{.07}$ & $\mstd{2.66}{.08}$  \\
 \midrule
ODMO$_{\text{NE}}$          & $\mstd{96.36}{.21}$  & $\mstd{0.17}{.01}$  & $\mstd{7.07}{.12}$ & $\mstd{2.52}{.05}$  \\
ODMO$_{\text{NE-MM}}$          & $\mstd{94.98}{.70}$  & $\mstd{0.16}{.01}$  & $\mstd{7.05}{.08}$ & $\mstd{2.71}{.03}$  \\
\bottomrule
\end{tabular}

\footnotesize
\centering
%\caption{\label{tab:mm_mocap}Benchmark for MM on Mocap  Dataset based on classifier.}
\begin{tabular}{@{}lcccc@{}}
\toprule
&\multicolumn{4}{c}{Mocap}   \\ \midrule
Methods                     & Acc$\uparrow$        & FID$\downarrow$     & Diversity          & MModality                   \\ \midrule
Real motions                & $\mstd{98.54}{.14}$  & $\mstd{0.02}{.00}$  & $\mstd{6.57}{.11}$ & $\mstd{2.17}{.08}$ \\ \midrule
ODMO                        & $\mstd{97.74}{.17}$  & $\mstd{0.09}{.00}$  & $\mstd{6.63}{.10}$ & $\mstd{2.07}{.10}$   \\

ODMO$_{\text{MM}}$  &    $\mstd{94.26}{.33}$  & $\mstd{1.02}{.06}$  & $\mstd{6.44}{.05}$ & $\mstd{2.63}{.09}$  \\
 \midrule
ODMO$_{\text{NE}}$          & $\mstd{87.30}{.51}$  & $\mstd{0.87}{.04}$  & $\mstd{6.33}{.10}$ & $\mstd{2.68}{.08}$  \\
ODMO$_{\text{NE-MM}}$          & $\mstd{85.58}{.90}$  & $\mstd{1.64}{.15}$  & $\mstd{6.26}{.07}$ & $\mstd{3.02}{.04}$  \\
 \bottomrule
\end{tabular}
\tiny
\begin{tabular}{@{}lccccc@{}}
\toprule
&\multicolumn{5}{c}{UESTC}   \\ \midrule
Methods                     & Acc$\uparrow$        & FID$_{tr}$ $\downarrow$ & FID$_{test}$$\downarrow$    & Diversity          & MModality                   \\ \midrule
Real motions                & $\mstd{99.79}{.05}$  & $\mstd{0.01}{.00}$              &       $\mstd{0.05}{.00}$                             & $\mstd{7.20}{.06}$ & $\mstd{1.61}{.02}$  \\ \midrule
ODMO                    & $\mstd{93.72}{.20}$ & $\mstd{0.18}{.03}$  &       $\mstd{0.21}{.00}$ & $\mstd{7.15}{.06}$ & $\mstd{1.80}{.03}$  \\

ODMO$_{\text{MM}}$  &    $\mstd{93.01}{.32}$  & $\mstd{0.16}{.00}$  & $\mstd{0.17}{.00}$  & $\mstd{7.12}{.05}$ & $\mstd{1.89}{.04}$  \\
 \midrule
ODMO$_{\text{NE}}$  &   $\mstd{91.52}{.50}$ & 
$\mstd{0.24}{.01}$ &    $\mstd{0.26}{.01}$ & 
$\mstd{7.13}{.07}$ & 
$\mstd{1.89}{.04}$  \\
ODMO$_{\text{NE-MM}}$          & $\mstd{89.86}{.16}$  & $\mstd{0.21}{.00}$  & $\mstd{0.22}{.01}$ & $\mstd{7.07}{.06}$ & $\mstd{2.12}{.03}$  \\
\bottomrule
\end{tabular}
\end{table}
